# Supplementary material for: Variation of Critical Crystallization Pressure for the Formation of Square Ice in Graphene Nanocapillaries
Source: arXiv:2307.03450 source file (2023-07-07)
Supplement: Supplementary file 1 [file Supporting_Information.pdf]

# Variation of Critical Crystallization Pressure for the Formation of Square Ice in Graphene Nanocapillaries: Supporting Information

Zhen Zeng[1], Kai Sun[1], Rui Chen[2], Mengshan Suo[1], Zhizhao Che[*1], and Tianyou Wang[†1]

[1]State Key Laboratory of Engines, Tianjin University, Tianjin, 300072, China.
[2]Department of Aeronautical and Automotive Engineering, Loughborough University, Loughborough LE11 3TU, United Kingdom.

July 5, 2023

[*]Corresponding author, Email: chezhizhao@tju.edu.cn
[†]Corresponding author, Email: wangtianyou@tju.edu.cn

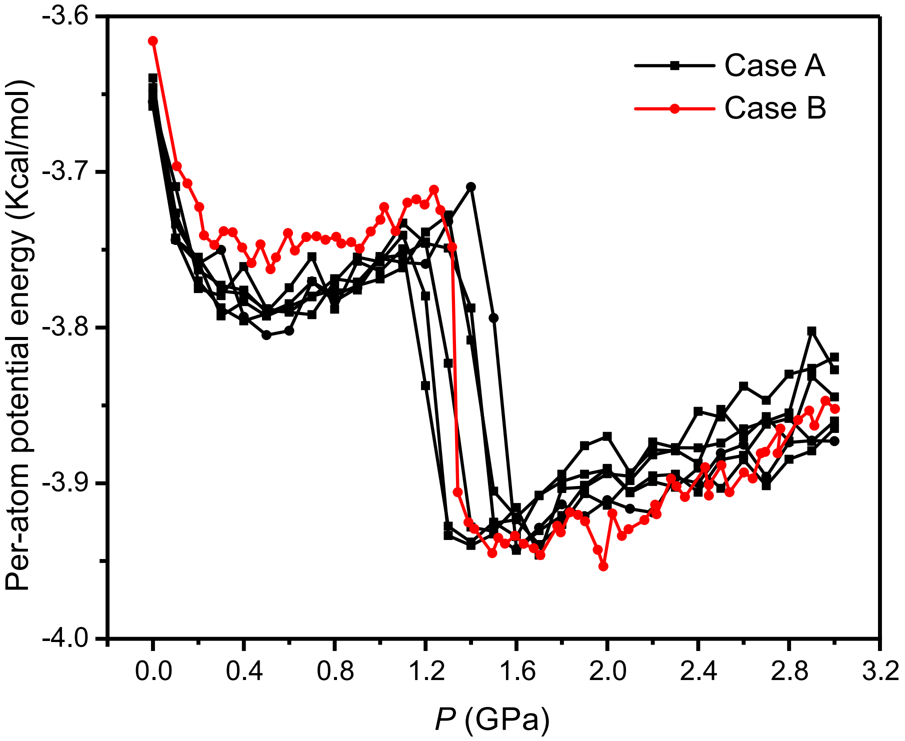


Figure S1: Variations of potential energy for repeated simulations with different initial velocities and different sizes of graphene sheets. Case A represents the results of typical size in this manuscript (42.5 Å × 35.0 Å for $D_z \times D_x$), and case B represents the results of a new size (42.5 Å × 21.9 Å for $D_z \times D_x$).

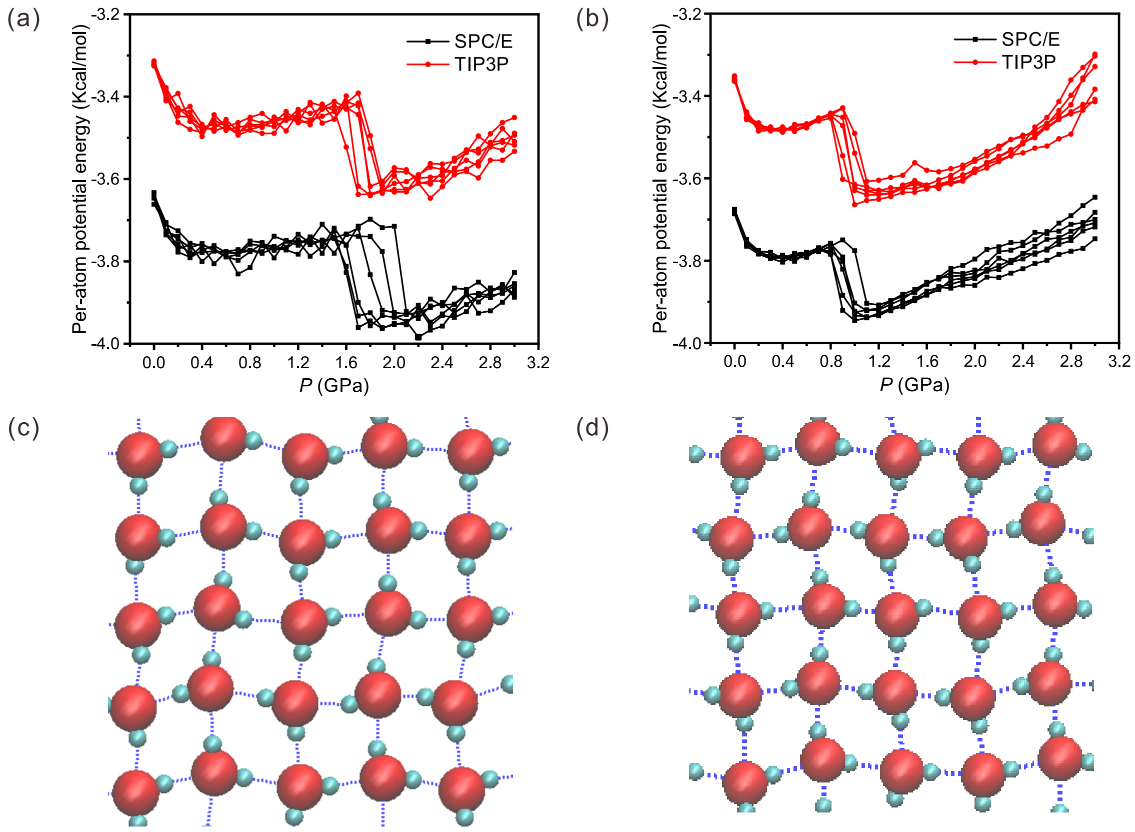


Figure S2: (a) Variation of the potential energy of the confined water during the pressurization process when the size of graphene sheets is 26.6 Å × 21.9 Å. (b) Variation of the potential energy of the confined water during the pressurization process when the size of graphene sheets is 68.0 Å × 56.0 Å. (c)–(d) Icing structures for TIP3P water model when the size of graphene sheets is 26.6 Å × 21.9 Å and 68.0 Å × 56.0 Å, respectively.

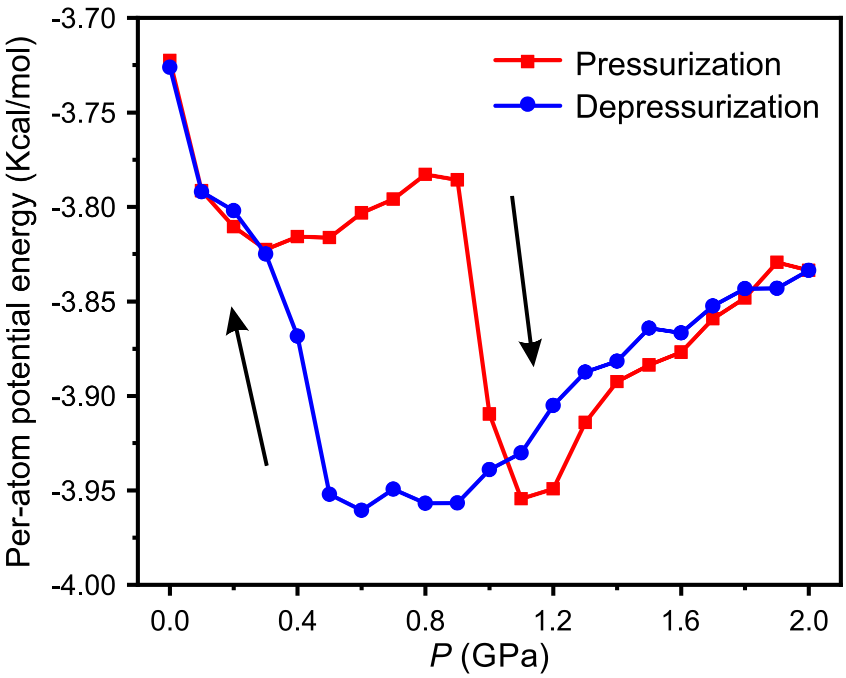


Figure S3: Pressurization/depressurization process (68.0 Å × 56.0 Å for $D_z \times D_x$).

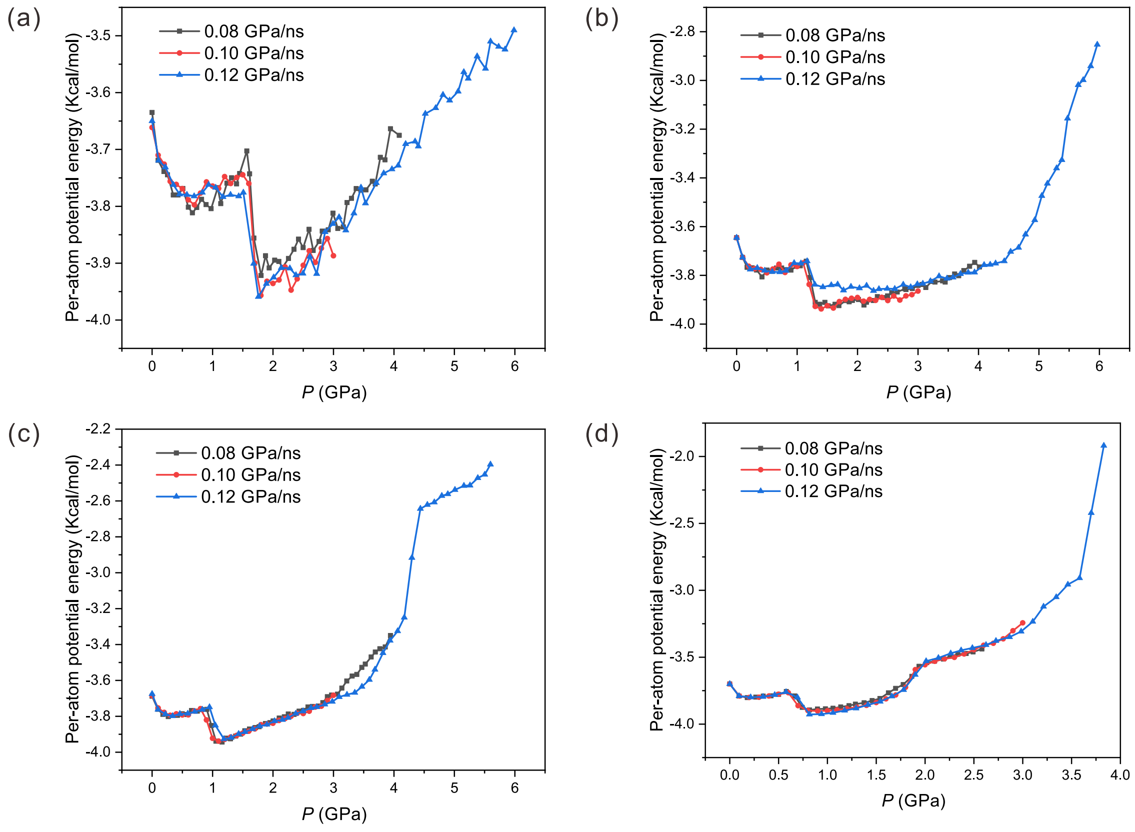


Figure S4: Variation of the potential energy of the confined water at different pressurization rates (0.08, 0.10, and 0.12 GPa/ns) during the pressurization process. (a)–(d) The size of graphene sheets is 26.6 Å × 21.9 Å, 42.5 Å × 35.0 Å, 68.0 Å × 56.0 Å, 108.8 Å × 89.6 Å, respectively.

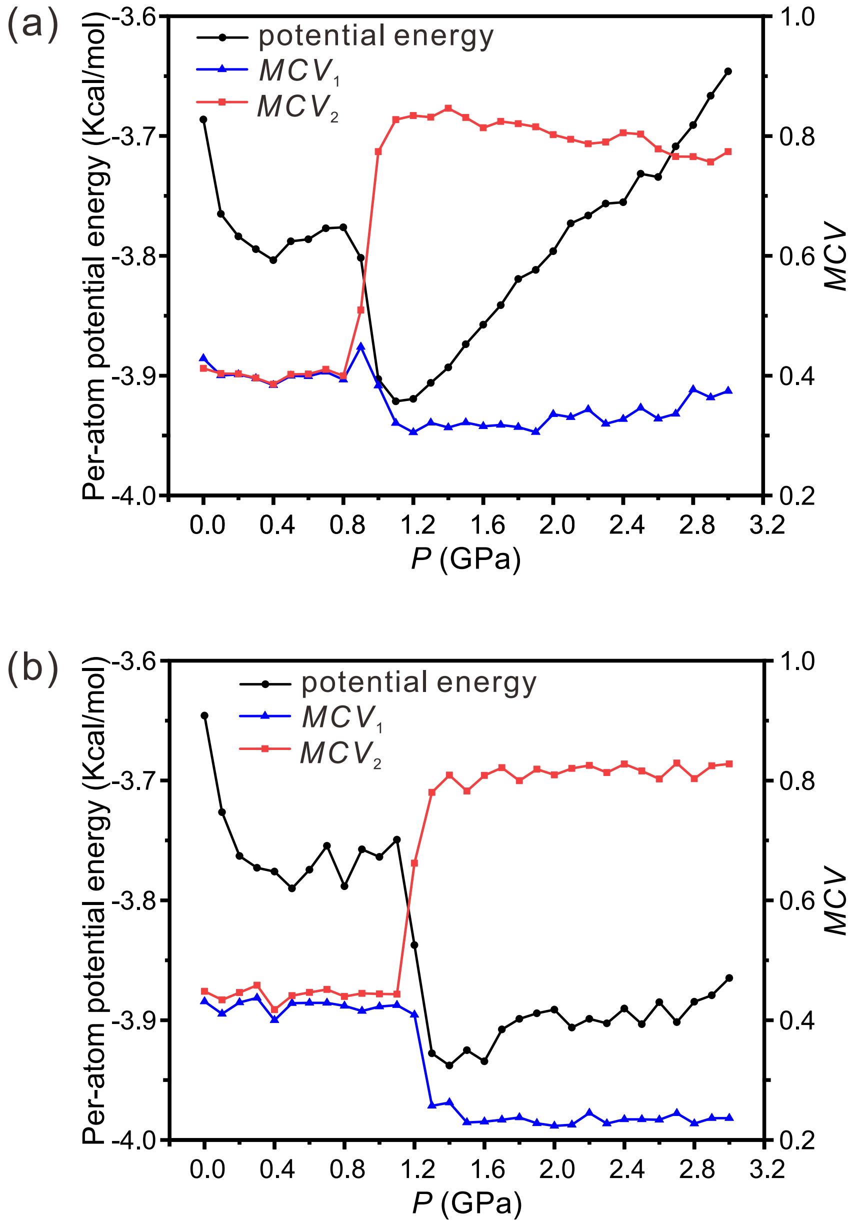


Figure S5: Variations of the per-atom potential energy and square icing parameters in the phase transformation of water molecules from liquid to ice by increasing the pressure. (a) 68.0 Å × 56.0 Å. (b) 42.5 Å × 35.0 Å.

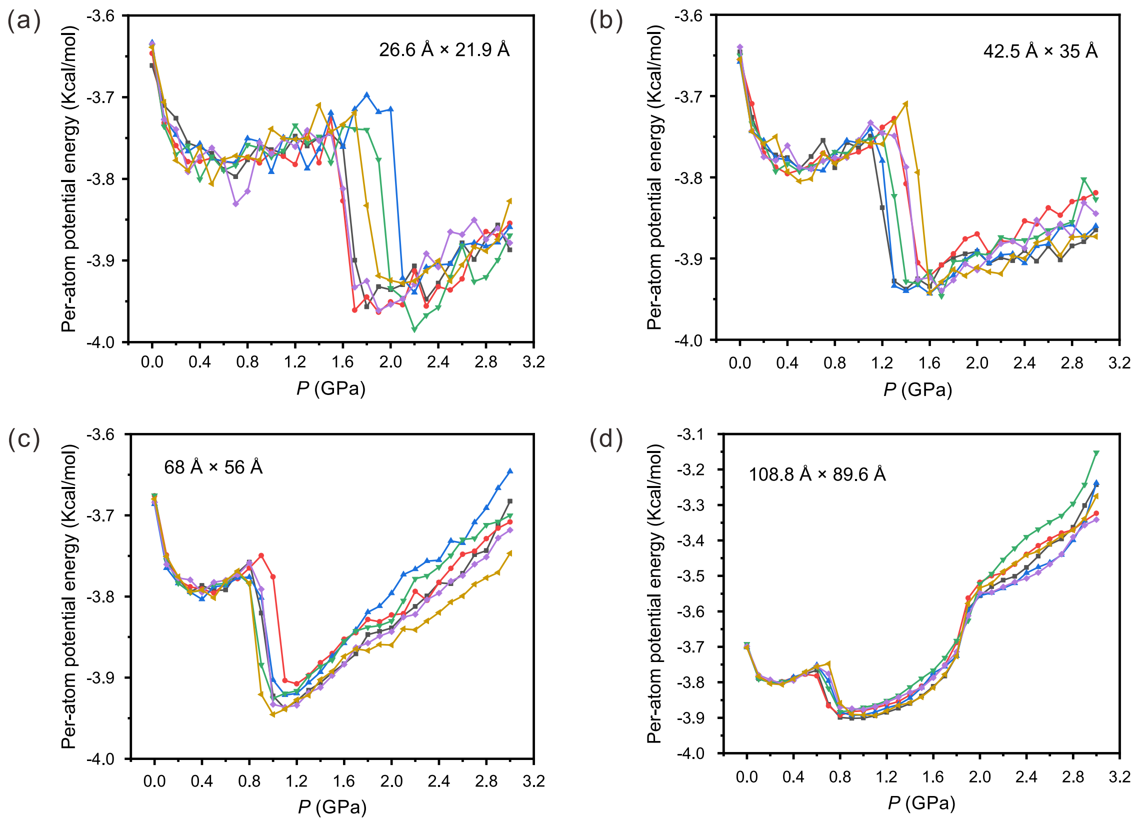


Figure S6: Variations of potential energy during the pressurization process for different cases when the size of graphene sheets is 26.6 Å × 21.9 Å, 42.5 Å × 35 Å, 68 Å × 56 Å, 108.8 Å × 89.6 Å, respectively.

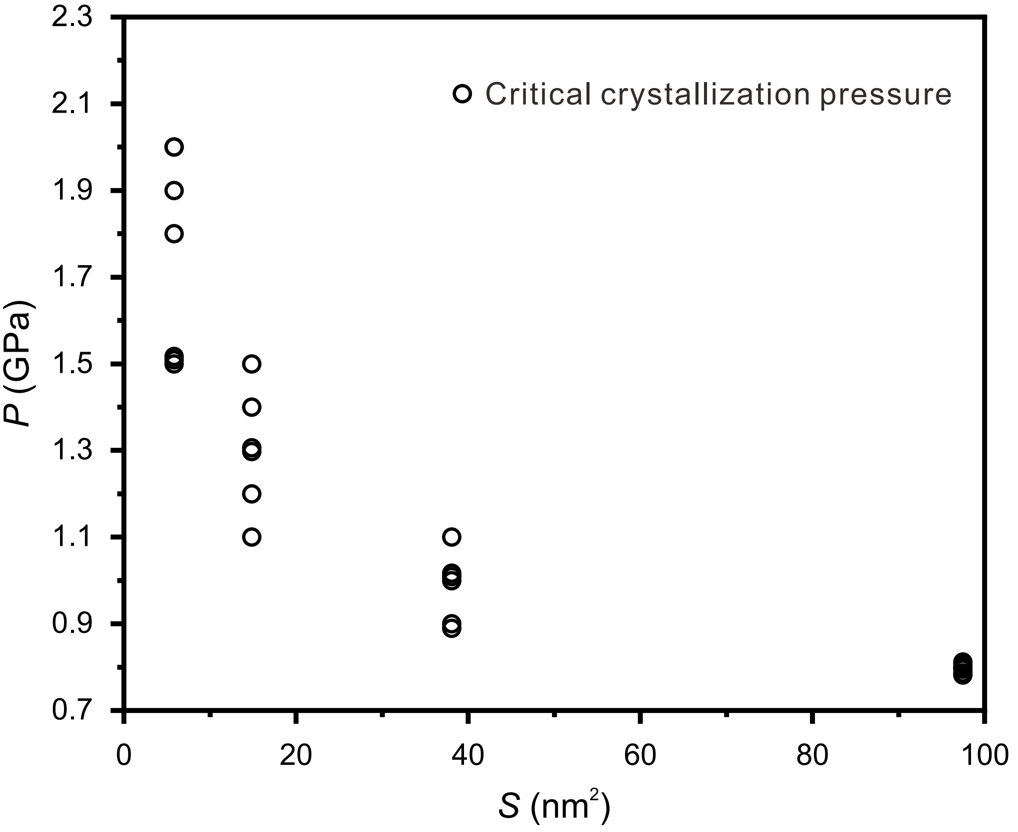


Figure S7: Distribution of critical crystallization pressure for all cases in Figure S7.

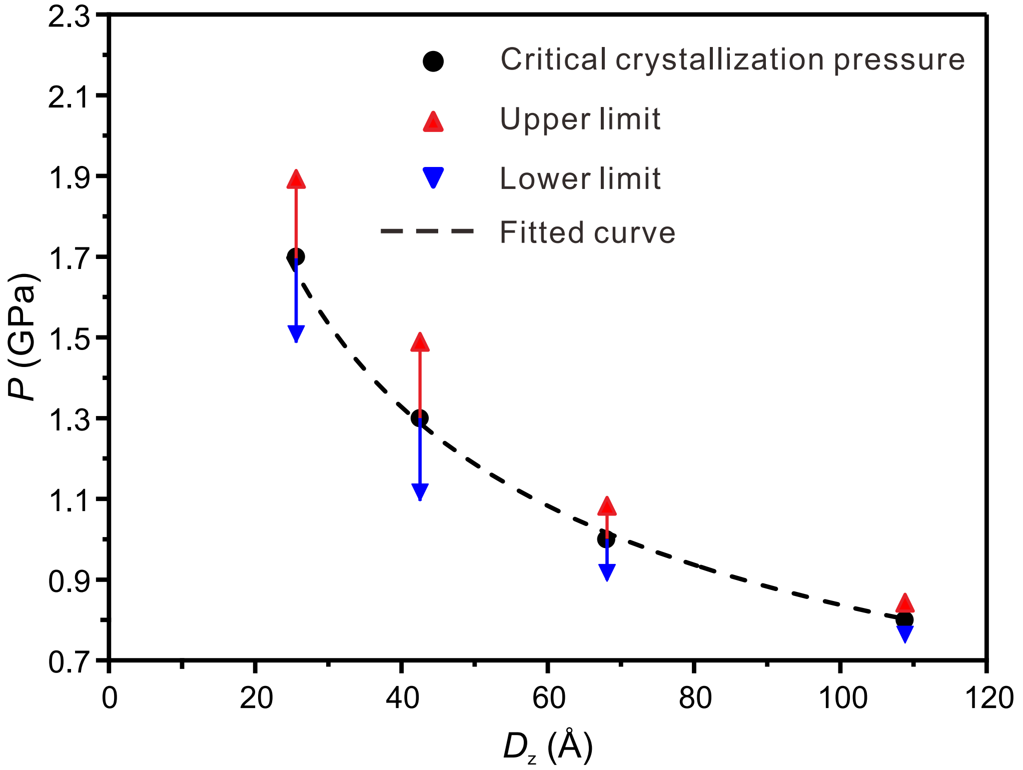


Figure S8: Critical crystallization pressure as a function of $D_z$. The red arrows represent the upper limit of critical crystallization pressure, the blue arrows represent the lower limit of critical crystallization pressure, the black dots represent the average critical crystallization pressure, and the black dashed curve is the fitted curve of the average critical crystallization pressure.

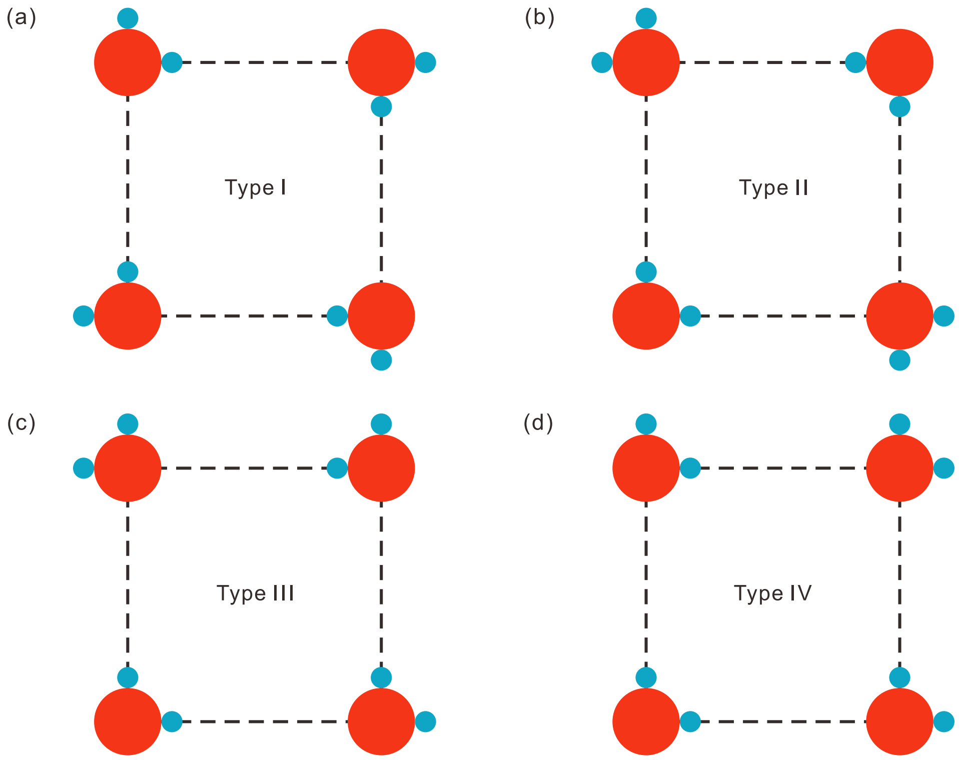


Figure S9: Sketches of detailed classification of the elementary units [2]. The red beads represent oxygen atoms, the cyan beads represent hydrogen atoms, and the black dashed lines represent hydrogen bonds. (a)–(b) Type I and type II units are the most common and "perfect", because there are no water molecules with the same arrangement in an elementary unit. (c) Type III unit has two synclastic water molecules at one side and the other two synclastic water molecules at another side. (d) The type IV unit has four synclastic water molecules.

# S1 Square Icing Parameters

To quantitatively determine and distinguish the partitioned square icing pattern from the homogeneous square icing pattern and the liquid water, square icing parameters, $MCV_1$ and $MCV_2$, are proposed in our previous works [1] and used in this study:

$$MCV_1 = \frac{1}{M} \sum_{m=1}^{M} \frac{\left[ \frac{1}{L} \sum_{l=1}^{L} \left( A_{lm} - \bar{A}_m \right)^2 \right]^{\frac{1}{2}}}{\bar{A}_m} \tag{S1}$$

$$MCV_2 = \frac{1}{L} \sum_{l=1}^{L} \frac{\left[ \frac{1}{M} \sum_{m=1}^{M} \left( A_{lm} - \bar{A}_l \right)^2 \right]^{\frac{1}{2}}}{\bar{A}_l} \tag{S2}$$

where $L$ and $M$ are two free positive integers, $l$ is an integer that runs from 1 to $L$, $m$ is an integer that runs from 1 to $M$, and $A_{lm}$ is the number of water molecules whose coordinate and orientation satisfy:

$$Z_{\min} + (l-1)\,(Z_{\max} - Z_{\min})/L \le z < Z_{\min} + l\,(Z_{\max} - Z_{\min})/L \tag{S3}$$

$$(m-1)\,\pi/(2M) \le \theta < m\pi/(2M) \tag{S4}$$

where $z$ is the coordinate of the water molecule in $z$ direction, $Z_{\min}$ and $Z_{\max}$ are the coordinate minimum and maximum of the graphene capillary in $z$ direction, respectively, and $\theta$ represents the direction of the hydrogen-oxygen bonds in the water molecule, which runs from $\theta = 0$ to $\theta = \pi/2$. The overbar in Eqs. (S1) and (S2) indicates the average, i.e.,

$$\bar{A}_m = \frac{1}{L} \sum_{l=1}^{L} A_{lm} \tag{S5}$$

$$\bar{A}_l = \frac{1}{M} \sum_{m=1}^{M} A_{lm} \tag{S6}$$

where $L = 13$ and $M = 18$ are chosen based on trials. $MCV_1 = 0.4$ and $MCV_2 = 0.6$ are taken as thresholds, from the data of many MD simulations. These square icing parameters analyze the uniformity of the distribution of water molecules in spatial position and direction of the hydrogen-oxygen bonds, so as to be able to identify the different phases and configurations of water molecules.

# References


[1] Zhen Zeng, Tianyou Wang, Rui Chen, Mengshan Suo, Kai Sun, Panagiotis E Theodorakis, and Zhizhao Che. Two-dimensional partitioned square ice confined in graphene/graphite nanocapillaries. *J. Chem. Phys.*, 156(15):154510, 2022.

[2] YinBo Zhu, FengChao Wang, and HengAn Wu. Structural and dynamic characteristics in monolayer square ice. *J. Chem. Phys.*, 147(4):044706, 2017.
